# Supplementary material for: Achieving Forgetting Prevention and Knowledge Transfer in Continual Learning
Source: arXiv:2112.02706 source file (2021-12-05)
Supplement: Supplementary file 1 [file suplementary.tex]

\documentclass{article}

% if you need to pass options to natbib, use, e.g.:
%     \PassOptionsToPackage{numbers, compress}{natbib}
% before loading neurips_2021

% ready for submission
\usepackage[final]{neurips_2021}

% to compile a preprint version, e.g., for submission to arXiv, add add the
% [preprint] option:
%     \usepackage[preprint]{neurips_2021}

% to compile a camera-ready version, add the [final] option, e.g.:
%     \usepackage[final]{neurips_2021}

% to avoid loading the natbib package, add option nonatbib:
%    \usepackage[nonatbib]{neurips_2021}
\usepackage{url}            % simple URL typesetting
\usepackage{booktabs}       % professional-quality tables
\usepackage{amsfonts}       % blackboard math symbols
\usepackage{nicefrac}       % compact symbols for 1/2, etc.
\usepackage{microtype}      % microtypography
\usepackage{subcaption}
\usepackage{amsmath,amsfonts,amssymb}
\usepackage{breqn}
\usepackage{tabularx}
\usepackage{multirow}
\usepackage{graphicx}
\usepackage{color}
\usepackage{tcolorbox}
\usepackage{CJK}
\usepackage{adjustbox}
\usepackage{xcolor}
\usepackage{colortbl}
\usepackage{multicol}
\usepackage{vwcol} 
\newsavebox{\algleft}
\newsavebox{\algright}
\usepackage{bm}
\usepackage{booktabs}
\usepackage{ctable} % for \specialrule command
\usepackage{amsmath,stackengine}
\usepackage[linesnumbered,ruled,vlined]{algorithm2e}
% Standard package includes
\usepackage{times}
\usepackage{latexsym}
\usepackage{bbm}
\usepackage[utf8]{inputenc} % allow utf-8 input
\usepackage[T1]{fontenc}    % use 8-bit T1 fonts
\usepackage{hyperref}       % hyperlinks
\usepackage{url}            % simple URL typesetting
\usepackage{booktabs}       % professional-quality tables
\usepackage{amsfonts}       % blackboard math symbols
\usepackage{nicefrac}       % compact symbols for 1/2, etc.
\usepackage{microtype}      % microtypography
\usepackage{xcolor}         % colors
\usepackage{array}
\newcolumntype{?}{!{\vrule width 1pt}}

\title{Supplemental Materials for \\ Achieving Forgetting Prevention and KnowledgeTransfer in Continual Learning} %\\
% Adapting BERT for Continual Learning of a Sequence of Aspect Sentiment Classification Tasks}

% The \author macro works with any number of authors. There are two commands
% used to separate the names and addresses of multiple authors: \And and \AND.
%
% Using \And between authors leaves it to LaTeX to determine where to break the
% lines. Using \AND forces a line break at that point. So, if LaTeX puts 3 of 4
% authors names on the first line, and the last on the second line, try using
% \AND instead of \And before the third author name.

\author{
Zixuan Ke$^{1}$, Bing Liu$^{1}$, Nianzu Ma$^{1}$, Hu Xu$^{2}$ and Lei Shu$^{3}$\thanks{Work was done prior to joining Amazon.} \\ 
$^1$Department of Computer Science, University of Illinois at Chicago\\
$^2$Facebook AI Research\\
$^3$Amazon AWS AI\\
$^1$\texttt{\{zke4,liub,nma4\}@uic.edu}\\  $^2$\texttt{huxu@fb.com} \\ $^3$\texttt{shulindt@gmail.com}
  % examples of more authors
  % \And
  % Coauthor \\
  % Affiliation \\
  % Address \\
  % \texttt{email} \\
  % \AND
  % Coauthor \\
  % Affiliation \\
  % Address \\
  % \texttt{email} \\
  % \And
  % Coauthor \\
  % Affiliation \\
  % Address \\
  % \texttt{email} \\
  % \And
  % Coauthor \\
  % Affiliation \\
  % Address \\
  % \texttt{email} \\
}
\begin{document}

\maketitle

\section{Task Masks (TM) in Task Specific Module (TSM)} %\zixuan{the task mask learning has been moved here} 
{\color{black}In this section, we detail the task mask (TM) training.
TMs (Figure~2(B) in the main paper) are used to prevent \textit{catastrophic forgetting} (CF), i.e., to protect the task specific knowledge of previous tasks.} Specifically, we first detect the neurons used by each old task, and then block off or mask out all the \textit{used} neurons when learning a new task. 

The task specific module (TSM) consists of %layers with 
%The key component in task specific module is the 
%task specific knowledge, which can be 
differentiable layers (CBA uses a 2-layer fully-connected network).
Each layer's output is further applied with a task mask to indicate which neurons should be protected for that task to overcome CF and forbids gradient updates for those neurons during backpropagation for a new task. 
Those tasks with overlapping masks indicate some parameter sharing. %\hu{to encourage knowledge sharing}.
%\hu{check if we can claim this or not} 
Due to KSM, the features flowing into those overlapping neurons enable the related old tasks to also improve in learning the new task.  % finds those neurons are also useful. % and supplies those neurons with shareable knowledge from KSM. 
% This allows for \textit{backward transfer}.

\textbf{Task Masks.}~Given the transfer capsule $v_j^{(t)}$, TSM maps them into input $k_l^{(t)}$ via a fully-connected network, where $l$ is the $l$-th layer in TSM. 
%During the mapping, the task specific module aims to learn features 
%neurons that are used by the previous tasks (\bing{?? what tasks?}) and blocking the gradient flow through the neurons (i.e., setting their gradients to 0). 
A task mask (a ``soft'' binary mask) ${m}^{(t)}_l$ is trained for each task $t$ at each layer $l$ in TSM during training task $t$'s classifier, indicating the neurons that are important for the task. Here we borrow the 
% \hu{this is another hard-attention different from routing? hard masking?} \zixuan{yes, this is a different hard attention technique, nothing to do with TR module}
hard attention idea in \cite{Serra2018overcoming} and leverage the task ID embedding to the train the task mask.

%\noindent \textbf{From Task ID Embedding to Task Mask.}
%\textbf{From Task ID to Task Specific Module. } 
% \hu{I moved from a previous paragraph.}
For a task ID $t$, its embedding $e^{(t)}_l$ consists of differentiable deterministic parameters that can be learned together with other parts of the network. 
%The subscript $l$ indicates the layer number. 
%A separate task ID embedding 
It is trained for each layer in TSM.
To generate the task mask $\text{m}^{(t)}_l$ from $e^{(t)}_l$, \textit{Sigmoid} is used as a pseudo-gate function and a positive %\hu{the formula seems can take negative too} 
scaling hyper-parameter $s$ is applied to help training. The $m^{(t)}_l$ is computed as follows:
%\vspace{-1.5mm}
\begin{equation}
% \vspace{-1.5mm}
\label{eq1}
m^{(t)}_l = \sigma(se^{(t)}_l).
\end{equation}
Note that the neurons in $m^{(t)}_l$ may overlap with those in other $m^{(i_{\text{prev}})}_l$'s from previous tasks showing some shared knowledge. Given the output of each layer in TSM, $k_l^{(t)}$, we element-wise multiply $k_l^{(t)} \otimes m^{(t)}_l$. The masked output of the last layer $k^{(t)}$ is fed to the next layer of the BERT with a skip-connection (Figure~1 {\color{black}in the main paper}). After learning task $t$, the final $m^{(t)}_l$ is saved and added to the set $\{m^{(t)}_l\}$. 

%\noindent \textbf{Block Gradients Flow through Used Neurons for Dissimilar Tasks.} 
\textbf{Training.}
For each past task $i_{\text{prev}} \in \mathcal{T}_{\text{prev}}$, its mask $m^{(i_{\text{prev}})}_l$ % is binary and conditions the training of task $i_{dis}$, 
indicates which neurons are used by that task and need to be protected. %$i_{\text{prev}}$. 
In learning task $t$, $m^{(i_{\text{prev}})}_l$ is used to set the gradient $g^{(t)}_l$ on \textit{all} used neurons of the layer $l$ in TSM to 0. Before modifying the gradient, we first accumulate all used neurons by all previous tasks' masks.
%making use of their masks. 
%\hu{not sure why binary can do accum. and other cannot, probably remove it?}
Since $m^{(i_{\text{prev}})}_l$ is binary, we use 
%element-wise maximum
max-pooling %\hu{is this just max-pooling?}
to achieve the accumulation:  
%\vspace{-1.5mm}
\begin{equation}
%\vspace{-1.5mm}
m^{(t_{\text{ac}})}_l = \text{MaxPool}(\{m^{(i_{\text{prev}})}_l\}).
\end{equation}

% \hu{it's better to replace tm to other variable: m?}
% \begin{equation}
% m^{(\leq i_{dis})}_l = max(m^{(i_{dis})}_l, m^{(\leq (r_{dis}^{(i-1)})}_l)
% \end{equation}

The term $m^{(t_{\text{ac}})}_l$ is applied to the gradient:
% \vspace{-1.5mm}
\begin{equation}
%\vspace{-1.5mm}
g^{'(t)}_l = g^{(t)}_l \otimes (1-m^{(t_{\text{ac}})}_l).
\end{equation}
Those gradients corresponding to the 1 entries in $m^{(t_{\text{ac}})}_l$ are set to 0 while the others remain unchanged. 
In this way, neurons in an old task are protected. 
%\hu{how a sharble knowledge from a similar/dissimilar task can use that or a new neurons?}\zixuan{The shareable knoweldge can use this becuase tasks are similar, otherwise it cannot}
Note that we expand (copy) the vector $m_l^{(t_{\text{ac}})}$ to match the dimensions of $g_l^{(t)}$.

Though the idea is intuitive, $e^{(t)}_l$ is not easy to train. To make the learning of $e^{(t)}_l$ easier and more stable, an annealing strategy is applied. %~\citep{Serra2018overcoming}. 
That is, $s$ is annealed during training, inducing a gradient flow and set $s=s_{\max}$ during testing. {\color{black}Eq.~\ref{eq1} approximates a unit step function as the mask, with $m_l^{(t)} \to \{0, 1\}$ when $s \to \infty$. 
A training epoch starts with all neurons being equally active, % with $s \to 0$, 
which are progressively polarized within the epoch. Specifically, $s$ is annealed as follows}:
% \vspace{-1.5mm}
\begin{equation}
%\vspace{-1.5mm}
\label{eq:smax}
s = \frac{1}{s_{\max}} + (s_{\max} - \frac{1}{s_{\max}})\frac{b-1}{B-1},
\end{equation}
where $b$ is the batch index and $B$ is the total number of batches in an epoch.

% \hu{put this directly in figure caption?}

% \textbf{Illustration.} The task masking process is illustrated in Figure~\ref{overview}(B), which shows the learning process of three tasks. Before training, those solid cells with a 0 are the neurons that have been used by some previous tasks and should be protected (masked). Those empty cells are free neurons (not used). After training, those solid cells with a 1 are neurons that are important for the current task, which will be used as masks in the future. Those solid cells with a 0 are masked as they are important for previous tasks. Those non-solid cells with a 0 are neurons that are not used so far.  % Note that those cells with multiple times 1 \bing{no multiple 1's} indicate that they are shared by more than one task.

Let us walk through the learning process of the three tasks in {\color{black}Figure~2(B) in the main paper}. After training task 0, we obtain its useful neurons indicated by the 1 entries. Before training task 1, those useful neurons for task 0 are first masked (those previous 1's entries are turned to 0's). After training task 1, two neurons with 1 are used by the task. When task 2 arrives, all used neurons by tasks 0 and 1 are masked before training, i.e., their entries are set to 0. After training task 2, we see that tasks 2 and 1 have a shared neuron (the cell with two colors, red and green), which is used by both of tasks. % We mark the shared neuron 1, although it has been used by task 0.

\section{Detailed Datasets Statistics}
\label{sec:dataset_detail}

% {In Section 5.1 of the main paper, we have described the task datasets for the document sentiment classification (DSC) application.} There is no additional information for DSC datasets to be provided. 
% \hu{I just shorten that as following} \bing{I make it longer as I want to give people the impression that the two applications are quite different.}
Since the datasets for the document sentiment classification (DSC) application (which is the same as a traditional classification problem) and the 20News dataset (which forms dissimilar task sequences and is used to show the forgetting avoidance ability) have already been described in Section 5.1 {\color{black}in the main paper, here we mainly focus on the datasets for} aspect sentiment classification (ASC), which is more than a traditional classification problem because of the additional input of the aspect and the fact that in the same sentence different aspects can have different opinions.  
% fine-grained and challenging. 
Table 1 in the main paper has provided the number of sentences or examples in each of the 19 datasets. However, no aspects or aspect opinions were provided. Here we provide them, %We detail the aspects and their associated opinions in the 19 datasets or tasks of ASC, 
as shown in
% are given in 
Table~\ref{tab:dataset}.

\begin{table*}[h]
\centering
\resizebox{\textwidth}{!}{
\begin{tabular}{ccccc}
\specialrule{.2em}{.1em}{.1em}
Dataset & Tasks/Domains & Training & Validating & Testing \\
\specialrule{.1em}{.05em}{.05em}

\multirow{3}{*}{Liu3domain} & Speaker & 233 S./352 A./287 P./65 N./0 Ne. & 30 S./44 A./35 P./9 N./0 Ne. & 38 S./44 A./40 P./4 N./0 Ne. \\
 & Router & 200 S./245 A./142 P./103 N./0 Ne. & 24 S./31 A./19 P./12 N./0 Ne. & 22 S./31 A./24 P./7 N./0 Ne. \\
 & Computer & 187 S./283 A./218 P./65 N./0 Ne. & 25 S./35 A./23 P./12 N./0 Ne. & 29 S./36 A./29 P./7 N./0 Ne. \\
\specialrule{.1em}{.05em}{.05em}
\multirow{5}{*}{HL5domain} & Nokia6610 & 209 S./271 A./198 P./73 N./0 Ne. & 29 S./34 A./30 P./4 N./0 Ne. & 28 S./34 A./25 P./9 N./0 Ne. \\
 & Nikon4300 & 131 S./162 A./135 P./27 N./0 Ne. & 15 S./20 A./18 P./2 N./0 Ne. & 15 S./21 A./19 P./2 N./0 Ne. \\
 & Creative & 582 S./677 A./422 P./255 N./0 Ne. & 68 S./85 A./42 P./43 N./0 Ne. & 70 S./85 A./52 P./33 N./0 Ne. \\
 & CanonG3 & 190 S./228 A./180 P./48 N./0 Ne. & 25 S./29 A./21 P./8 N./0 Ne. & 24 S./29 A./24 P./5 N./0 Ne. \\
 & ApexAD & 281 S./343 A./146 P./197 N./0 Ne. & 35 S./43 A./16 P./27 N./0 Ne. & 28 S./43 A./31 P./12 N./0 Ne. \\
\specialrule{.1em}{.05em}{.05em}
\multirow{9}{*}{Ding9domain} & CanonD500 & 103 S./118 A./96 P./22 N./0 Ne. & 11 S./15 A./14 P./1 N./0 Ne. & 13 S./15 A./11 P./4 N./0 Ne. \\
 & Canon100 & 137 S./175 A./123 P./52 N./0 Ne. & 19 S./22 A./20 P./2 N./0 Ne. & 16 S./22 A./21 P./1 N./0 Ne. \\
 & Diaper & 166 S./191 A./143 P./48 N./0 Ne. & 22 S./24 A./18 P./6 N./0 Ne. & 24 S./24 A./22 P./2 N./0 Ne. \\
 & Hitachi & 152 S./212 A./153 P./59 N./0 Ne. & 23 S./26 A./19 P./7 N./0 Ne. & 23 S./27 A./14 P./13 N./0 Ne. \\
 & Ipod & 124 S./153 A./101 P./52 N./0 Ne. & 18 S./19 A./14 P./5 N./0 Ne. & 19 S./20 A./15 P./5 N./0 Ne. \\
 & Linksys & 152 S./176 A./128 P./48 N./0 Ne. & 19 S./22 A./13 P./9 N./0 Ne. & 20 S./23 A./16 P./7 N./0 Ne. \\
 & MicroMP3 & 384 S./484 A./340 P./144 N./0 Ne. & 42 S./61 A./48 P./13 N./0 Ne. & 51 S./61 A./39 P./22 N./0 Ne. \\
 & Nokia6600 & 298 S./362 A./244 P./118 N./0 Ne. & 26 S./45 A./32 P./13 N./0 Ne. & 39 S./46 A./30 P./16 N./0 Ne. \\
 & Norton & 168 S./194 A./54 P./140 N./0 Ne. & 17 S./24 A./15 P./9 N./0 Ne. & 24 S./25 A./5 P./20 N./0 Ne. \\
\specialrule{.1em}{.05em}{.05em}
\multirow{2}{*}{SemEval14} & Rest & 1893 S./3452 A./2094 P./779 N./579 Ne. & 84 S./150 A./70 P./26 N./54 Ne. & 600 S./1120 A./728 P./196 N./196 Ne. \\
 & Laptop & 1360 S./2163 A./930 P./800 N./433 Ne. & 98 S./150 A./57 P./66 N./27 Ne. & 411 S./638 A./341 P./128 N./169 Ne. \\
\specialrule{.1em}{.05em}{.05em}

\end{tabular}
}
\caption{Statistics of the ASC datasets. \textbf{S}.: number of sentences; \textbf{A}: number of aspects; \textbf{P., N., and Ne.}: number aspects with 
positive, negative and neutral opinions, respectively. Note that the SemEval14 datasets have 3 classes of opinion polarities (positive, negative and neutral) while the others have only 2 classes (positive and negative) because in these other datasets, those sentences with neutral opinions were not annotated with aspects and thus cannot be used in \textit{aspect} sentiment classification (ASC). %as they have no annotated aspects\zixuan{"as they have no annotated aspects" seems duplicated} , 
That is why we have ``0 Ne.'' for those datasets.  %\zixuan{We cannot use those sentences without sentiment (neutral) in 2-classes datasets for aspect sentiment classification (ASC) \bing{are you sure the 2-class datasets are not used, but only the 3-class datasets, so only two tasks for ASC?} because they were not annotated with aspects in the original data in these datasets,}. %Note that while we can regard all the un-annotated review sentence as neutral polarity, they are still lack of aspect annotated.\bing{I thought these other datasets also have three classes. Is it that these other datasets do not have aspect annotation when there is no sentiment?}\zixuan{yes}
}
\label{tab:dataset}
\end{table*}

\section{Standard Deviations}
% \zixuan{We use p-value previously, we are changing it to std} 
We report the standard deviations (Table 2) of the accuracy (Acc.) and macro-F1 (MF1) results of CTR and the considered baselines over 5 runs with random seeds {\color{black}based on one random task sequence used in the paper. Note that {this is different from Table 2 of the main paper where }each result reported is the average result of 5 random task sequences as different task sequences can produce different results.} We can see the results of CTR are stable. Some baselines can have quite large standard deviations using Adapter-BERT.

% To show that our results from BACK are significantly
% better than those of baselines, we conduct a paired t-test. We test BACK against each of the baselines based on their final results. All p-values are below 0.05 (see Table \ref{tab:significant_test}), which indicates that CTR is significantly better than every baseline. % \zixuan{Now everyone is less than 0.05}

% \zixuan{one may also consider percentage}

\begin{table}[h!]
\centering
\resizebox{\columnwidth}{!}{
\begin{tabular}{ccc||cccccccc}
\specialrule{.2em}{.1em}{.1em}
\multirow{2}{*}{Scenarios} & \multirow{2}{*}{Category} & \multirow{2}{*}{Model} & \multicolumn{2}{c}{{ASC}} & \multicolumn{2}{c}{{DSC (small)}} & \multicolumn{2}{c}{{DSC (full)}} & \multicolumn{2}{c}{{20News}} \\
 &  &  & {Acc.} & {MF1} & {Acc.} & {MF1} & {Acc.} & {MF1} & {Acc.} & {MF1} \\ \specialrule{.1em}{.05em}{.05em}
\multirow{4}{*}{\begin{tabular}[c]{@{}c@{}}Non-continual   \\      Learning (SDL)\end{tabular}} & \multicolumn{1}{l}
{BERT} & MTL &	$\pm${0.0073} &	$\pm${0.0088} &	$\pm${0.0111} &	$\pm${0.0117} &	$\pm${0.0034} &	$\pm${0.0037} &	$\pm${0.0049} &	$\pm${0.0049}\\
& \multicolumn{1}{l}{BERT} & SDL & $\pm${0.0118} & $\pm${0.0263} & $\pm${0.0288} & $\pm${0.0401} & $\pm${0.0048} & $\pm${0.0052} & $\pm${0.0022} & $\pm${0.0022} \\
  & BERT (Frozen) & SDL & $\pm${0.0171} & $\pm${0.0265} & $\pm${0.0019} & $\pm${0.0027} & $\pm${0.0042} & $\pm${0.0063} & $\pm${0.0044} & $\pm${0.0044} \\
 & \multicolumn{1}{l}{Adapter-BERT} & SDL  & $\pm${0.0175} & $\pm${0.0154} & $\pm${0.0081} & $\pm${0.0150} & $\pm${0.0053} & $\pm${0.0060} & $\pm${0.0048} & $\pm${0.0048} \\
 & \multicolumn{1}{l}{W2V} & SDL & $\pm${0.0102} & $\pm${0.0077} & $\pm${0.0082} & $\pm${0.0131} & $\pm${0.0072} & $\pm${0.0094} & $\pm${0.0022} & $\pm${0.0022} \\

 \cline{1-11}
\multirow{25}{*}{\begin{tabular}[c]{@{}c@{}}Continual \\      Learning (CL)\end{tabular}} & \multicolumn{1}{l}{BERT} & NFH  & $\pm${0.1051} & $\pm${0.0492} & $\pm${0.0274} & $\pm${0.0363} & $\pm${0.0736} & $\pm${0.0701} & $\pm${0.0518} & $\pm${0.0508} \\
 & BERT (Frozen) & NFH  & $\pm${0.0042} & $\pm${0.0098} & $\pm${0.0023} & $\pm${0.0040} & $\pm${0.0051} & $\pm${0.0049} & $\pm${0.0044} & $\pm${0.0045} \\ 
 & \multicolumn{1}{l}{Adapter-BERT} & NFH & $\pm${0.0659} & $\pm${0.0885} & $\pm${0.0801} & $\pm${0.0608} & $\pm${0.0792} & $\pm${0.0923} & $\pm${0.0396} & $\pm${0.0677} \\
 & \multicolumn{1}{l}{W2V} & NFH & $\pm${0.0133} & $\pm${0.0325} & $\pm${0.0064} & $\pm${0.0206} & $\pm${0.0203} & $\pm${0.0337} & $\pm${0.0132} & $\pm${0.0146} \\  
 \cline{2-11}
 & \multirow{6}{*}{BERT   (frozen)}
 & L2 & $\pm${0.0618} & $\pm${0.0405} & $\pm${0.0320} & $\pm${0.0134} & $\pm${0.0358} & $\pm${0.0731} & $\pm${0.0161} & $\pm${0.0230} \\
 &  & A-GEM & $\pm${0.0078} & $\pm${0.0142} & $\pm${0.0036} & $\pm${0.0036} & $\pm${0.0037} & $\pm${0.0042} & $\pm${0.0037} & $\pm${0.0037} \\
  &  & DER++ & $\pm${0.0067} & $\pm${0.0077} & $\pm${0.0056} & $\pm${0.0060} & $\pm${0.0135} & $\pm${0.0160} & $\pm${0.0530} & $\pm${0.0759} \\
 &  & KAN & $\pm${0.0099} & $\pm${0.0170} & $\pm${0.0348} & $\pm${0.0361} & $\pm${0.0088} & $\pm${0.0089} & $\pm${0.0335} & $\pm${0.0432} \\
 &  & SRK & $\pm${0.0105} & $\pm${0.0175} & $\pm${0.0184} & $\pm${0.0230} & $\pm${0.0052} & $\pm${0.0059} & $\pm${0.0247} & $\pm${0.0318} \\
 &  & EWC & $\pm${0.0714} & $\pm${0.0392} & $\pm${0.0154} & $\pm${0.0368} & $\pm${0.0329} & $\pm${0.0398} & $\pm${0.0509} & $\pm${0.0808} \\
 &  & UCL  & $\pm${0.0205} & $\pm${0.0477} & $\pm${0.0053} & $\pm${0.0053} & $\pm${0.0046} & $\pm${0.0047} & $\pm${0.0048} & $\pm${0.0048} \\
 &  & OWM & $\pm${0.0165} & $\pm${0.0206} & $\pm${0.0002} & $\pm${0.0027} & $\pm${0.0174} & $\pm${0.0078} & $\pm${0.0139} & $\pm${0.0144} \\
 &  & HAT & $\pm${0.0209} & $\pm${0.0304} & $\pm${0.0146} & $\pm${0.0200} & $\pm${0.0047} & $\pm${0.0065} & $\pm${0.0423} & $\pm${0.0567} \\
 &  & CAT & $\pm${0.0246} & $\pm${0.0649} & $\pm${0.0584} & $\pm${0.1012} & $\pm${0.0103} & $\pm${0.0097} & $\pm${0.0067} & $\pm${0.0068}\\

 \cline{2-11}
 & \multirow{4}{*}{Adapter-BERT} & L2 & $\pm${0.0313} & $\pm${0.0499}  & $\pm${0.0766} & $\pm${0.1237} & $\pm${0.0383} & $\pm${0.0449} & $\pm${0.0278} & $\pm${0.0374}\\
 &  & A-GEM & $\pm${0.0941} & $\pm${0.0609} & $\pm${0.0934} & $\pm${0.1319} & $\pm${0.0624} & $\pm${0.0662} & $\pm${0.0235} & $\pm${0.0318} \\
  &  & DER++ & $\pm${0.0853} & $\pm${0.0712} & $\pm${0.0813} & $\pm${0.1195} & $\pm${0.1005} & $\pm${0.0963} & $\pm${0.0984} & $\pm${0.1161} \\
 &  & EWC & $\pm${0.0943} & $\pm${0.0991} & $\pm${0.0610} & $\pm${0.0831} & $\pm${0.1209} & $\pm${0.1215} & $\pm${0.0409} & $\pm${0.0616} \\
 &  & UCL  & $\pm${0.0731} & $\pm${0.0341} & $\pm${0.0436} & $\pm${0.0203} & $\pm${0.1017} & $\pm${0.1022} & $\pm${0.1322} & $\pm${0.0890} \\
 &  & OWM & $\pm${0.0347} & $\pm${0.0419} & $\pm${0.0381} & $\pm${0.0344} & $\pm${0.0046} & $\pm${0.0044} & $\pm${0.0316} & $\pm${0.0461} \\
 &  & HAT & $\pm${0.0058} & $\pm${0.0091}  &  $\pm${0.0112} & $\pm${0.0119} & $\pm${0.0197} & $\pm${0.0205} & $\pm${0.0037} & $\pm${0.0037}\\
 \cline{2-11}

 & \multirow{6}{*}{W2V} & L2 & $\pm${0.0124} & $\pm${0.0078} & $\pm${0.0116} & $\pm${0.0233} & $\pm${0.0252} & $\pm${0.0157} & $\pm${0.0128} & $\pm${0.0219}  \\
 &  & A-GEM & $\pm${0.0062} & $\pm${0.0238} & $\pm${0.0164} & $\pm${0.0301} & $\pm${0.0191} & $\pm${0.0250} & $\pm${0.0076} & $\pm${0.0086}  \\
  &  & DER++ & $\pm${0.0059} & $\pm${0.0130} & $\pm${0.0249} & $\pm${0.0415} & $\pm${0.0163} & $\pm${0.0219} & $\pm${0.0140} & $\pm${0.0148} \\
 &  & KAN & $\pm${0.0111} & $\pm${0.0044} & $\pm${0.0083} & $\pm${0.0162} & $\pm${0.0473} & $\pm${0.0302} & $\pm${0.0067} & $\pm${0.0065} \\
 &  & SRK  & $\pm${0.0074} & $\pm${0.0029} & $\pm${0.0161} & $\pm${0.0162} & $\pm${0.0031} & $\pm${0.0057} & $\pm${0.0123} & $\pm${0.0151} \\
 &  & EWC  & $\pm${0.0264} & $\pm${0.0581} & $\pm${0.0478} & $\pm${0.0952} & $\pm${0.0155} & $\pm${0.0208} & $\pm${0.0412} & $\pm${0.0424} \\
 &  & UCL & $\pm${0.0148} & $\pm${0.0110} & $\pm${0.0056} & $\pm${0.0131} & $\pm${0.0209} & $\pm${0.0313} & $\pm${0.0113} & $\pm${0.0121} \\
 &  & OWM & $\pm${0.0258} & $\pm${0.0299} & $\pm${0.0228} & $\pm${0.0348} & $\pm${0.0167} & $\pm${0.0194} & $\pm${0.0196} & $\pm${0.0249} \\
 &  & HAT & $\pm${0.0194} & $\pm${0.0203} & $\pm${0.0192} & $\pm${0.0220} & $\pm${0.0484} & $\pm${0.0553} & $\pm${0.0422} & $\pm${0.0700}  \\
 & &  CAT & $\pm${0.0114} & $\pm${0.0278} & $\pm${0.0001} & $\pm${0.0002} & $\pm${0.0182} & $\pm${0.0242} & $\pm${0.0251} & $\pm${0.0317} \\
 \cline{2-11}
& \multicolumn{2}{c||}{B-CL}
&  $\pm${0.0093} & $\pm${0.0324} & $\pm${0.0177} & $\pm${0.0208} & $\pm${0.0111} & $\pm${0.0117} & $\pm${0.0085} & $\pm${0.0087} \\
& \multicolumn{2}{c||}{LAMOL}  & $\pm${0.0256} & $\pm${0.0085} &	$\pm${0.0089} & $\pm${0.0241} &	$\pm${0.0316} & $\pm${0.0300} &	$\pm${0.0254} & $\pm${0.0265} \\ \cline{2-8}
 & \multicolumn{2}{c||}{CTR} &  $\pm${0.0107} & $\pm${0.0123} & $\pm${0.0083} & $\pm${0.0076} & $\pm${0.0011} & $\pm${0.0016} &  $\pm${0.0067} & $\pm${0.0067}
% 0.0107 0.0123	0.0083	0.0076	0.0011	0.0016	0.0067	0.0067
\\
\specialrule{.1em}{.05em}{.05em}

\end{tabular}
}
\caption{{\color{black}Standard deviations of the accuracy (Acc.) and Macro-F1 (MF1) results of the proposed CTR model and the baselines on the four experiments.} % \zixuan{added MTL, LAMOL and B-CL column}
% \bing{In table 2 of the main paper the first two rows for 20News have no results, how come there are results here?}  %\zixuan{Note: the highest one can be around 0.15}
% \hu{rename Adapter to Adapter-MLP ? }
% \hu{summarize the effects of knowledge transfer and forgetting? do we need statistical testing?}
\vspace{-4mm}
} 
%The number in bold in each row is the best result of the row.}
% \hu{
% it seems how to use the embeddings are not important but how to do CL is more important; (re-group into NL/NFH with different sub-rows? 
%TODO: add citation to each baseline if possible.)
%}
\label{tab:std_results}
\end{table}

\section{Execution Time and Number of Parameters}

% \zixuan{This table has been enlarged}
% \zixuan{Training time is tricky since it is related to a lot of factors, need to somehow normalized them}
Table \ref{tab:parameter_time} reports the number of parameter (regardless of trainable or non-trainable), training execution times for different models. The execution time is computed as the average training time \textit{per task}. 
% The testing time is computed as the total testing time for all tasks after all tasks are learned sequentially. 
Our experiments were run on GeForce GTX 2080 Ti with 11G GPU memory.

\begin{table}[h!]
\centering
\resizebox{\columnwidth}{!}{
\begin{tabular}{ccc||c?cccc}
\specialrule{.2em}{.1em}{.1em}
\multirow{2}{*}{Scenarios} & \multirow{2}{*}{Category} & \multirow{2}{*}{Model} & \multirow{2}{*}{\#Parameters (M)} & \multicolumn{4}{c}{Running time (min)} \\
 &  &  &  & \multicolumn{1}{l}{ASC} & DSC (small) & DSC (full) & 20News\\
 \specialrule{.1em}{.05em}{.05em}
\multirow{4}{*}{\begin{tabular}[c]{@{}c@{}}Non-continual   \\      Learning (SDL)\end{tabular}} & \multicolumn{1}{l}{BERT} & MTL & 109.5 & 1.3 & 0.8 & 19.1 & 3.4  \\
& \multicolumn{1}{l}{BERT} & SDL & 109.5 & 2.1 & 1.7 & 23.8 & 4.9  \\
  & BERT (Frozen) & SDL & 110.4 &  3.3  & 3.2 & 17.3 & 7.0\\
 & Adapter-BERT & SDL & 183.3 & 5.1 & 3.4 & 32.8 & 6.4 \\
 & W2V & SDL & 6.7 & 0.7 &0.2 &0.6 & 0.5 \\
 \cline{1-8}
\multirow{21}{*}{\begin{tabular}[c]{@{}c@{}}Continual \\      Learning (CL)\end{tabular}} 
 & BERT & NFH & 109.5 & 2.1 & 1.7 & 23.8 & 4.9 \\
 & BERT (Frozen) & NFH & 110.4 &  3.3  & 3.2 & 17.3 & 7.0 \\
 & Adapter-BERT & NFH & 183.3 & 5.1 & 3.4 & 32.8 & 6.4\\
 & W2V & NFH & 6.7 & 0.7 &0.2 &0.6 & 0.5  \\ 
 \cline{2-8}
 & \multirow{10}{*}{BERT   (frozen)}  & L2 & 110.4 & 3.4 & 2.5 & 17.6 & 7.4\\
 &  & A-GEM* & 110.4 & 3.3  & 3.2 & 17.3 & 7.0\\
 &  & DER++* & 110.4 & 3.3 & 3.2 & 17.3 & 7.0\\
 & & KAN & 116.6 &  1.4 & 1.0 & 7.5 & 1.9\\
 &  & SRK & 117.8 & 3.3 & 8.8 & 35.9 & 7.1  \\
 &  & EWC & 110.4 & 5.7 & 2.6 & 29.7 & 12.4\\
 &  & UCL & 110.4 & 3.4 & 2.0 & 17.2 & 7.2\\
 &  & OWM & 110.6 & 3.4 & 2.0 & 17.1 & 7.2\\
 &  & HAT & 111.3 & 3.4 & 2.0 & 17.4 & 7.3\\ 
 &  & CAT & 227.4 & 23.8 & 23.0 & 124.56 & 50.4\\
 \cline{2-8}

 & \multirow{7}{*}{Adapter-BERT} & L2 & 183.3 & 2.7 & 2.5 & 31.7 & 6.5\\
 &  & A-GEM* & 183.3 & 5.1 & 3.4 & 32.8 & 6.4\\
  &  & DER++* & 183.3 & 5.1 & 3.4 & 32.8 & 6.4\\
 &  & EWC & 183.3 & 4.8 & 3.9 & 60.3 & 12.3\\
 &  & UCL & 183.4 &  2.3 & 2.2 & 26.8 & 5.5\\
 &  & OWM & 184.4 & 2.7 &  2.6 & 30.1 & 6.2\\
 &  & HAT & 185.2 & 2.7 & 2.5 & 30.3 & 6.2\\  \cline{2-8}

 & \multirow{10}{*}{W2V} & L2 & 6.2 & 8.2 & 0.2 & 0.6 & 0.5\\
 &  & A-GEM* & 6.2 &  0.7 &0.2 & 0.6 & 0.5  \\ 
 &  & DER++* & 6.2 & 0.7 &0.2 & 0.6 & 0.5  \\ 
 &  & KAN & 7.0 & 0.1 &0.1 & 0.2 & 0.1\\
 &  & SRK & 7.2  & 2.4 & 2.8 & 3.1 & 4.2\\
 &  & EWC & 6.2 & 1.2  & 0.4 & 3.0 & 1.4 \\
 &  & UCL & 6.2 & 0.7  & 0.3 & 0.7 & 0.5\\
 &  & OWM & 6.4  & 0.7  & 0.2 & 0.8 & 0.5\\
 &  & HAT & 6.4 & 0.8  & 0.3 & 1.0 & 0.6  \\ 
 &  & CAT & 24.5 & 5.0 & 1.4 & 4.5 & 3.6 \\
 \cline{2-8}
  & \multicolumn{2}{c||}{B-CL} & 287.4 & 27.8 & 14.5 & 90.2 & 35.1 \\
  & \multicolumn{2}{c||}{LAMOL} & 124.4 & 7.2 & 6.0 & 18.0 & 24.0  \\ \cline{2-8}
 & \multicolumn{2}{c||}{CTR} & 223.1 & 65.9	& 26.0 & 131.6 & 87.3 \\
\specialrule{.1em}{.05em}{.05em}
\end{tabular}
}
\caption{Network size (\#parameters in millions, regardless of trainable or non-trainable) and average training time per task of each model measured in minutes. {\color{black} We use ``*'' to indicate a replay method with a memory buffer. Here we report \#parameters without including the memory buffer. %We store 5\% of the examples for each tasks in the buffer. 
{\color{black}The extra parameters and more training time used by our system} % \bing{correct?}\zixuan{"extra parameters and training time in our system"}
are mainly due to the use of capsules and adapters. 
} %\zixaun{added MTL, LAMOL and B-CL column}
%\ls{why adapter bert ewc dsc (full) running time is that high, BERT frozen SDL DSC full that low? Readers may assume there are some trends or consistency inside the running time, for example, method1 take fewer time in DSC small than method 2, then method 1 takes fewer time in DSC full than method 2. However, I observe DSC full breaks the consistency. Maybe we can explain the phenomenon if we use early stopping or other methods}\zixuan{EWC can be time consuming due to the computation of Fisher Information. We do use early stopping in BERT (frozen) and W2C, while BERT and Adapter-BERT we use a fixed number of training epochs. I feel like the training time of different training strategy is not quite comparable.}
\vspace{-4mm}
} 
\label{tab:parameter_time}
\end{table}

\section{Hyperparameter Search}
%\zixuan{Adapted from CLASSIC, remove "validation results"}
%Sec.~5.3 in the main paper reported the best hyper-parameters. 
{\color{black}We use grid search to find the best parameters based on the validation data performance. We search within \{32, 64, 128\} for batch size, within \{140, 200, 300, 400\} for $s_{max}$, within \{300, 768, 2000\} for dimension of Task Specific Module (TSM) and within \{10, 20, 30, 40\} for the number of BERT training epochs.
All reported test results in the paper are given by the parameters with the best validation performance.} % We encourage the reviewers and interested readers to play with the submitted code.

\bibliography{neurips_2021}
\bibliographystyle{abbrv}

\end{document}
