# Supplementary material for: Achieving Forgetting Prevention and Knowledge Transfer in Continual Learning
Source: arXiv:2112.02706 source file (2021-12-05)
Supplement: Supplementary file 2 [file icml2021_author_response.tex]

\documentclass{article}

% Please use the following line and do not change the style file.
\usepackage{icml2021_author_response}

% Recommended, but optional, packages for figures and better typesetting:
\usepackage{microtype}
\usepackage{graphicx}
\usepackage{subfigure}
\usepackage{hyperref}       % hyperlinks
\usepackage{booktabs} % for professional tables
\usepackage{amsfonts}       % blackboard math symbols
\usepackage{nicefrac}       % compact symbols for 1/2, etc.
\usepackage{lipsum}
\usepackage{subcaption}
\usepackage{amsmath,amsfonts,amssymb}
\usepackage{breqn}
\usepackage{tabularx}
\usepackage{multirow}
\usepackage{graphicx}
\usepackage{color}
\usepackage{tcolorbox}
\usepackage{CJK}
\usepackage{adjustbox}
\usepackage{xcolor}
\usepackage{colortbl}
\usepackage{multicol}
\usepackage{vwcol} 
\newsavebox{\algleft}
\newsavebox{\algright}
\usepackage{bm}
\usepackage{booktabs}
\usepackage{ctable} % for \specialrule command
\usepackage{amsmath,stackengine}
\usepackage{wrapfig}

\newcommand{\zixuan}[1]{{\color{blue}{\small\bf\sf [zixuan: #1]}}}
\newcommand{\bing}[1]{{\color{red}{\small\bf\sf [bing: #1]}}}
\newcommand{\hu}[1]{{\color{orange}{\small\bf\sf [hu: #1]}}}
\newcommand{\ls}[1]{{\color{magenta}{\small\bf\sf [lei: #1]}}}

\begin{document}
% Uncomment the following line if you prefer a single-column format
%\onecolumn
Thank you (R1, R3, R5, R6) for your insightful comments. We will fix all minor issues and cite all suggested papers.

\textbf{[R1] Additional baselines GEM and L2.}
\vspace{-2mm}
% \begin{table}[]
\begin{wraptable}{r}{0cm}
\centering
\resizebox{0.8\columnwidth}{!}{%
\begin{tabular}{cccccc}
\specialrule{.2em}{.1em}{.1em} 
\multirow{2}{*}{Category} & \multicolumn{1}{c}{\multirow{2}{*}{Model}} & \multicolumn{2}{c}{ASC} & \multicolumn{2}{c}{DSC} \\
 & \multicolumn{1}{c}{} & Acc. & MF1 & Acc. & MF1 \\
\specialrule{.1em}{.05em}{.05em} 
\specialrule{.1em}{.05em}{.05em} 
\multirow{2}{*}{BERT (Frozen)} & L2 & 0.5604 & 0.3840 & 0.5917 & 0.4839 \\
 & GEM & 0.7660 & 0.6022 & 0.7730 & 0.7154 \\
 \specialrule{.1em}{.05em}{.05em}
\multirow{2}{*}{Adapter-BERT} & L2 & 0.6397 & 0.5243 & 0.6726 & 0.6276 \\
 & GEM &  0.8378 & 0.7357  & 0.8325  & 0.8213 \\
 \specialrule{.1em}{.05em}{.05em}
\multicolumn{2}{c}{\textbf{BACK}} & \textbf{0.8947} & \textbf{0.8362} & \textbf{0.8434} & \textbf{0.8329} \\
\specialrule{.1em}{.05em}{.05em} 
\vspace{-9mm}
\end{tabular}
}
% \caption{Experiments with Suggested Baselines}
\caption{Two more baselines: GEM and L2}
\vspace{-6mm}
\label{tab:suggested_baselines}
\end{wraptable}
% \end{table}

\vspace{-2mm}
We did not use GEM as it
is a replay method that stores previous task data. BACK does not store any data. 
L2 is not used as we have 
% \hu{GEM solves a different problem that compresses previous task data into a generator, whereas the problem for BACK does not allow to save past data for CL, as in Table 3. (check if my statement is correct)} 
% already included 
more powerful baselines. 
% We have run them and give the results in Table 3, which shows BACK is dramatically better. 
Table 1 shows that BACK outperforms GEM and L2. We will implement the EWC variant in the revision. % We agree that it is still interesting to see how BACK perform comparing to these two baselines. We follow the publicly available code to get their performance (for GEM, we set 128 buffer size and 5\% replay ratio).

\textbf{[R1, R3, R5]: The masks will grow and limit the number of tasks to be learned.} % Fortunately, 
This is not an issue as neurons have significant sharing across tasks (a masked neuron cannot be updated by a new task but can be used by the new task). The network size can be increased on-the-fly. It does not affect the old tasks, which are protected by task masks. % \zixuan{(R5) If a neuron has been masked in Task 1, how can it be trained in Task 2, as shown in Fig 1(B)? }

\textbf{[R3, R6]: BACK vs. KAN, SRK and Adapter-BERT.}
% \hu{I think the problem is different, you are using pre-trained large-scale model, then how to leverage big pre-trained model, right?}
Although KAN and SRK can perform knowledge transfer as BACK, BACK also deals with forgetting which KAN and SRK cannot (see the next response). Even for knowledge transfer, BACK outperforms both KAN and SRK by a large margin. Note, we have applied BERT (frozen; KAN and SRK cannot use Adapter) to KAN and SRK (originally use word vectors) to make them better. The BACK model is also totally different. KAN or SRK does not use capsules and cannot use Adapter-BERT. Our transfer routing is also designed specifically for transfer, which is different from existing routing methods used in capsules. % KAN and SRK do not use BACK aims to tackle CL problems under the well-known pre-training/fine-tuning scheme and it is non-trivial to fine-tune BERT in CL.
We are unaware of BERT adapter being used for continual learning (CL). We developed an effective adapter CBA for CL. % which leveraging CapsuleNet that is completely different from adapter-BERT \hu{why mention they save parameter? which was proposed to save parameters (??).}
%, but they are still much poorer than BACK. % do not perform better than 

% (1) KAN or SRK does not use capsule network, or BERT, and cannot use adapter-BERT. Our transfer routing method is also designed specifically for transfer, which is different from existing routing methods used in capsules. 
% (2) It is none trivial to apply continual learning (CL) to BERT as fine-tuning BERT causes serious forgetting. 
% We are unaware of any report of BERT adapter being used for continual learning. Our adapter CBA is completely different from the original adapter in adapter-BERT, which was proposed to save parameters (??). (3) BACK outperforms both KAN and SRK by large margins. Note that we have applied BERT (frozen; they cannot use Adapter) to the original KAN and SRK (which use word vectors (W2V)) to make them perform better, but they are still much poorer than BACK. % do not perform better than without CL, i.e., their knowledge transfer is not effective.

% all considered baselines when applying them to BERT.
% \vspace{-3mm}
% \begin{table}[]
\begin{wraptable}{r}{0cm}
\centering
% \vspace{-3mm}
\resizebox{0.5\columnwidth}{!}{%
\begin{tabular}{cccc}
\specialrule{.2em}{.1em}{.1em} 
\multicolumn{1}{c}{\multirow{2}{*}{Category}} & \multicolumn{1}{c}{\multirow{2}{*}{Model}} & \multicolumn{2}{c}{20NG} \\
\multicolumn{1}{c}{} & \multicolumn{1}{c}{} & Acc. & MF1 \\
\specialrule{.1em}{.05em}{.05em} 
\specialrule{.1em}{.05em}{.05em} 
BERT & SDL & 0.9649 & 0.9648 \\
Adapter-BERT & SDL & 0.9620 & 0.9619 \\
%\specialrule{.1em}{.05em}{.05em}
%BERT & NFH & 0.5250 & 0.3922 \\
%Adapter-BERT & NFH & 0.6829 & 0.6170 \\
\specialrule{.1em}{.05em}{.05em}
\multirow{2}{*}{BERT (Frozen)} & KAN & 0.7307 & 0.6997 \\
 & SRK & 0.7964	 &  0.7789 \\
%  & EWC & 	 &   \\
\specialrule{.1em}{.05em}{.05em}
\multirow{1}{*}{Adapter-BERT} 
%  & L2 & 0.6956 &  0.6550 \\
%  & GEM & 0.6419	 &  0.5367 \\
 & HAT & 0.9522 & 0.9521 \\
\specialrule{.1em}{.05em}{.05em}
% \multicolumn{2}{c}{LAMOL} & 0.6613 & 0.4574 \\
\multicolumn{2}{c}{\textbf{BACK}} & \textbf{0.9525} & \textbf{0.9523}\\
\specialrule{.1em}{.05em}{.05em} 
\vspace{-9mm}
\end{tabular}
}
% \caption{Experiments with Unrelated Domains}
\caption{Unrelated tasks}
\vspace{-6mm}
\label{tab:20ng}
\end{wraptable}
% \end{table}
\textbf{[R3]: Related and unrelated domain or domain shifted tasks.} The paper showed BACK can transfer knowledge and avoid forgetting for related/similar domain tasks, which is {the} main goal of our paper. To ensure that BACK also works for unrelated domain tasks, we ran BACK, KAN and SRK on 20Newgroup (20NG) data, which is a topic classification dataset with no or little shared knowledge across tasks. Thus, our goal is to achieve \textit{no or little forgetting}. %Since domains are unrelated, there is nothing much to transfer among task. As a result, the SDL becomes the upper bound since no forgetting can happen under this setting. To prepare the task sequence, we use 20NewsGroup (20NG) to evaluate BACK with unrelated domains. 
We split the 20 classes of 20NG into 10 tasks with 2 classes per task. Compared to single domain learning (SDL), Table~\ref{tab:20ng} shows BACK actually performs equally well as HAT. HAT uses masks to protect each task and thus has almost no forgetting. Thus, BACK is suitable for both related and unrelated tasks. KAN and SRK have serious forgetting. % only slightly poor than the upper bound (SDL). Comparing with the best baseline (HAT), which almost does not forget. BACK is actually slightly better. 

\textbf{[R3, R5] Clarity of CBA.} We thank you for pointing out many minor clarity issues. We look at them all carefully. All can be addressed easily. Due to space limitations, we will have to clarify them and improve the writing in the revised paper.  In Eq. 4, $a_{j|t}^{(t)}$ is a typo and it should be $a_{j|i}^{(t)}$.
% Eq.~1 generates task capsules from input feature $h^{(t)}$. Assume $d_k$ is the dimension of capsule $i$, $p_i^{(t)}\in\mathbb{R}^{d_t\times d_k}$. 
 % as the similarity is computed between every previous task and current task. We will make it clear that 
% $*$ refers to the convolution operation and
% $a_{j|i}^{(t)}$ contains the output of all filters and $\otimes$ refers to element-wise multiplication. The similarity computation is inspired by (Xue \& Liu, 2018). We will also try other similarity scoring in the future. 


\begin{wraptable}{r}{0cm}
\centering
\resizebox{0.5\columnwidth}{!}{%
\begin{tabular}{cccc}
\specialrule{.2em}{.1em}{.1em} 
\multicolumn{1}{c}{\multirow{2}{*}{Category}} & \multicolumn{1}{c}{\multirow{2}{*}{Model}} & \multicolumn{2}{c}{DSC-larger} \\
\multicolumn{1}{c}{} & \multicolumn{1}{c}{} & Acc. & MF1 \\
%\specialrule{.1em}{.05em}{.05em} 
%\specialrule{.1em}{.05em}{.05em} 

%BERT & SDL & 0.8784 & 0.8680 \\
%Adapter-BERT & SDL & 0.8830 & 0.8731 \\
%\specialrule{.1em}{.05em}{.05em}
%BERT & NFH & 0.7308 & 0.7181 \\
%Adapter-BERT & NFH & 0.6494 & 0.6340 \\
\specialrule{.1em}{.05em}{.05em}
\multicolumn{1}{c}{\multirow{3}{*}{BERT (Frozen)}} & KAN & 0.8232 & 0.8123 \\
\multicolumn{1}{c}{} & SRK & 0.8399 & 0.8266 \\
\multicolumn{1}{c}{} & EWC &  0.7277 &	0.6576\\
\specialrule{.1em}{.05em}{.05em}
Adapter-BERT & HAT & 0.8800 & 0.8726 \\
\specialrule{.1em}{.05em}{.05em}
\multicolumn{2}{c}{\textbf{BACK}} & \textbf{0.8931} & \textbf{0.8875}\\
\specialrule{.1em}{.05em}{.05em} 
\vspace{-9mm}
\end{tabular}
}
% \caption{Experiments with larger DSC datasets}
\caption{KAN's full data}
\vspace{-6mm}
\label{tab:larger_dsc}
\end{wraptable}
% \end{table}
\textbf{[R6] KAN's full data.} The paper used only 400 training examples in each task in KAN's dataset to show that BACK is superior as labeling training data is expensive, and when the training data is small, transfer is usually more effective. KAN's original dataset has 4000 training examples per task. We have run BACK with all 4000 examples in each task. % experimented with the full data, %We compare BACK with SDL, NFH, KAN, SRK and the best existing baseline HAT. We can see in 
Table~\ref{tab:larger_dsc} shows that BACK still outperforms baselines (due to space limits, we only show 4 strongest baselines), although slightly less than the 400 setting in the paper because with a large amount of labeled data in each task, cross-task knowledge transfer is less necessary.   

% \begin{table}[]
\begin{wraptable}{r}{0cm}
\centering
\resizebox{0.7\columnwidth}{!}{%
\begin{tabular}{cccccc}
\specialrule{.2em}{.1em}{.1em} 
\multicolumn{1}{c}{\multirow{2}{*}{\begin{tabular}[c]{@{}c@{}}Category  \\ (BERT-large)\end{tabular}}} & \multicolumn{1}{c}{\multirow{2}{*}{Model}} & \multicolumn{2}{c}{ASC} & \multicolumn{2}{c}{DSC} \\
\multicolumn{1}{c}{} & \multicolumn{1}{c}{} & Acc. & MF1 & Acc. & MF1 \\
\specialrule{.1em}{.05em}{.05em} 
\specialrule{.1em}{.05em}{.05em} 
BERT & SDL & 0.8683 & 0.7853 & 0.8450 & 0.8237 \\
Adapter-BERT & SDL & 0.8532	& 0.7428 & 0.8362 & 0.8179 \\
%\specialrule{.1em  }{.05em}{.05em}
%BERT & NFH & 0.5809 & 0.5246 & 0.5930 & 0.5425 \\
%Adapter-BERT & NFH &  0.6282 & 0.5538 & 0.6620 & 0.6185  \\
\specialrule{.1em}{.05em}{.05em}
BERT (Frozen) & EWC & 0.8483 & 0.7229 & 0.8321 & 0.7748   \\
Adapter-BERT & HAT & 0.8748 & 0.7986 & 0.8416 & 0.8264 \\
\specialrule{.1em}{.05em}{.05em}
\multicolumn{2}{c}{\textbf{BACK}} &  \textbf{0.8943} & \textbf{0.8250}  & \textbf{0.8604} & \textbf{0.8495} \\
\specialrule{.1em}{.05em}{.05em} 
\vspace{-9mm}
\end{tabular}
}
% \caption{Experiments with Unrelated Domains}
\caption{Using BERT-large}
\vspace{-4mm}
\label{tab:bert_large}
\end{wraptable}
% \end{table}

\textbf{[R6] BERT-large.} The paper used BERT-base. We have run BERT-large. EWC and HAT are two strongest baselines. 
%We showed Bert-based has difficulty in knowledge transfer and suffering from CF. To check whether this is because the limited number of parameters, we further evaluate BACK under BERT-large setting. In 
Table~\ref{tab:bert_large} shows that BACK still outperforms the baselines by large margins. %  comparing SDL and NFH, we can see the forgetting is still server in BERT-large setting (even more server than BERT-based). 

% \textbf{\#Parameters(R1,R4).}
\textbf{Other Comments:}
% We will show progressive results to show the effectiveness of BACK in terms of forgetting avoidance and knowledge transfer.
\textbf{(R3)} Baselines in Table 2 in the paper use the same datasets and the scores are recomputed as EWC, UCL, OWM and HAT are for images and have to be adapted for text.~KAN and SRK did not use BERT (BERT performs better). %We believe the proposed adapter-based approach can be applied to other pre-trained models. 
We will add the 2 new references. Although the ICML-2020 paper deals with forgetting and transfer, it is for unsupervised topic modeling. Our adapter should be applicable to other pretrained models. \textbf{(R5)} Ablation shows the most effective components are TSM (task specific module) and TR (task router). %We also improve the description of CBA. 
\textbf{(R6)} Although LAMOL paper showed that GPT-2 is more powerful than BERT, we ran LAMOL on the ASC data and got lower accuracy 0.8891 and MF1 0.8059 (BACK accuracy 0.8947 and MF1 0.8362). LAMOL also suffers from forgetting on 20NG data. Its accuracy is only 0.6613, much worse than 0.9525 of BACK. Network sizes are given in Supplementary. For those BERT based methods, the BERT parameters (109.5M) are also included. Most Task-CL methods don't do well as they are designed for dealing with forgetting but we need knowledge transfer. \textbf{(All Reviewers)} Due to space limits, we will address all minor issues in the revised paper. % fail to improve or even degrades the performance of baseline %We agree that it is still interesting to see whether BACK can work well comparing to LAMOL. We evaluate LAMOL using the sequence of ASC dataset by running the author provided code (5\% replay ratio). %LAMOL is not direct comparable with BACK as it uses GPT-2, which has been shown in the LAMOL paper to be much stronger than BERT (which we use). % which is what BACK and other baselines based on. % In its paper, the author shows GPT-2 is powerful enough to outperform BERT-based model by a large margin; 



% \zixuan{(R3) how would the proposed approach apply to other net-works, not based on BERT architecture}

% \zixuan{(R6) why is BACK(-KSM;-TSM)equivalent to Adapter-BERT? }

% \zixuan{(R6) it seems confusing to see that most existing Task-CL methods fail to improve or even degrades the performance of baseline}
% We also tried to decrease the number of parameters of BACK Experiments show that we can use 160.9M parameters and achieve the same performance.

% \lipsum
% \lipsum
\end{document}
